# Supplementary material for: Entropic Unmixing in Nematic Blends of Semiflexible Polymers
Source: arXiv:2009.06271 source file (2020-09-14)
Supplement: Supplementary file 1 [file SI.pdf]

# Supporting Information: Entropic Unmixing in Nematic Blends of Semiflexible Polymers

Andrey Milchev,[1,2] Sergei A. Egorov,[3,2] Jiarul Midya,[2] Kurt Binder,[2] and Arash Nikoubashman[2]
[1]*Institute for Physical Chemistry, Bulgarian Academia of Sciences, 1113 Sofia, Bulgaria*
[2]*Institute of Physics, Johannes Gutenberg University Mainz, Staudingerweg 7, 55128 Mainz, Germany*
[3]*Department of Chemistry, University of Virginia, Charlottesville, VA 22901, USA*
(Dated: September 14, 2020)

## I. MODEL DETAILS

### A. Molecular Dynamics

In our Molecular Dynamics (MD) simulations, excluded volume interactions between monomeric units, each with diameter $\sigma$, are taken into account through the Weeks-Chandler-Andersen (WCA) potential[1]

$$U_{\rm m}(r) = \begin{cases} 4\varepsilon\left[\left(\frac{\sigma}{r}\right)^{12} - \left(\frac{\sigma}{r}\right)^{6}\right] + \varepsilon, & r \leq 2^{1/6}\sigma \\ 0, & r > 2^{1/6}\sigma \end{cases}, \quad (1)$$

where $r$ is the center-to-center distance between a pair of monomers, and $\varepsilon$ sets the energy scale for the repulsion. These interactions correspond to good solvent conditions for dilute polymer solutions.

Polymer bonds are included through the finitely extensible nonlinear elastic (FENE) potential

$$U_{\rm b}(r) = \begin{cases} -\frac{kr_0^2}{2}\ln\left[1 - \frac{r^2}{r_0^2}\right], & r \leq r_0 \\ \infty, & r > r_0 \end{cases}, \quad (2)$$

with spring constant $k = 30\,\varepsilon/\sigma^2$ and maximum bond length $r_0 = 1.5\,\sigma$ to prevent unphysical chain crossing.[2] The equilibrium bond length is then $\ell_{\rm b} = 0.97\,\sigma$.

Bending stiffness is included through

$$U_{\rm bend}(\theta_{ijk}) = \kappa\left[1 - \cos\left(\theta_{ijk}\right)\right] \approx \frac{\kappa}{2}\theta_{ijk}^2, \quad (3)$$

where $\theta_{ijk}$ is the bond angle formed by the bond vectors $\mathbf{a}_i = \mathbf{r}_j - \mathbf{r}_i$ and $\mathbf{a}_j = \mathbf{r}_k - \mathbf{r}_j$, with $\mathbf{r}_i$, $\mathbf{r}_j$, and $\mathbf{r}_k$ being the positions of successive monomeric units $i$, $j$, and $k$. Then one can show that the bond orientational correlations $\langle \mathbf{a}_i \cdot \mathbf{a}_{i+s}\rangle \propto \exp(-s\ell_{\rm b}/\ell_{\rm p})$, for $s = 1, 2, 3, \ldots$ and $s\ell_{\rm b} \ll \ell_{\rm p}$. Note that $\ell_{\rm p} \approx \ell_{\rm b}\kappa/(k_{\rm B}T)$ for $\kappa \gtrsim 2\,k_{\rm B}T$ and at densities below the isotropic-nematic transition,[3] as expected from the equipartition theorem ($T$ being the absolute temperature, and $k_{\rm B}$ the Boltzmann constant).

### B. Calculation of polymer excluded volume

Our Density Functional Theory (DFT) calculations require information on the excluded volume between two (semiflexible) polymers, $V_{\rm excl}$, at a given relative orientation $\gamma$. Fynewever and Yethiraj determined $V_{\rm excl}$ by performing Monte Carlo (MC) simulations of tangent hard sphere chains consisting of $N$ monomers with diameter $\sigma$.[4] Bending stiffness was introduced through Eq. (3). In Ref. 4, $V_{\rm excl}$ was computed for pairs of chains with equal length, $N_{\rm A} = N_{\rm B} = N$, and equal stiffness, $\kappa_{\rm A} = \kappa_{\rm B} = \kappa$, and we used those data to determine the average excluded volume $V_{\rm excl}^{\rm avg}(\gamma) = (V_{\rm excl}^{\rm AA} + V_{\rm excl}^{\rm BB})/2$ (see the inset of Fig. 1 in the main manuscript).

In this work, we followed the same approach to compute $V_{\rm excl}$ for cases where $\kappa_{\rm A} \neq \kappa_{\rm B}$. To this end, we generated 500 different pairs of chains using the continuum configurational bias method.[5] Then, we computed the molecular axis of each chain using the eigenvector corresponding to the smallest eigenvalue of the moment of inertia tensor, and rotated the chains to a fixed relative angle $\gamma$. The excluded volume is then determined by moving one chain relative to the other one for $N_{\rm move} = 10^5$ times, and counting the number of moves, $N_{\rm overlap}$, that resulted in an overlap of at least one monomer. The excluded volume between the chains is then given by

$$V'_{\rm excl} = V_{\rm box}N_{\rm overlap}/N_{\rm move}, \quad (4)$$

where $V_{\rm box}$ is the volume of the cubic simulation box with edge length $L_{\rm box} = 2N\sigma$. This procedure is then repeated for relative orientations ranging from 0 to $\pi/2$ in steps of $\pi/12$. To interpolate between these points, we fit the resulting data to the function[4]

$$V_{\rm excl}(\gamma) = c_1 + c_2\left(1 - c_3\cos^2\gamma\right)^{1/2} \quad (5)$$

with fitting constants $c_1$, $c_2$, and $c_3$, which are summarized in Table I for the systems studied in our work.

| $\kappa_{\rm A}$ | $\kappa_{\rm B}$ | $c_1$ | $c_2$ | $c_3$ |
|---|---|---|---|---|
| 16 | 16 | 548.0 | 260.8 | 0.913 |
| 128 | 128 | 179.2 | 752.6 | 0.949 |
| 16 | 128 | 367.4 | 499.7 | 0.8768 |
| 20 | 128 | 387.6 | 486.9 | 0.9388 |
| 24 | 128 | 323.9 | 561.5 | 0.8988 |

TABLE I. Fitting parameters for $V_{\rm excl}$ given in Eq. (5) for $N = 32$. The values for $\kappa_{\rm A} = \kappa_{\rm B}$ have been adapted from Ref. 4.

To provide a qualitative explanation why the effective excluded volume between a pair of semiflexible poly-

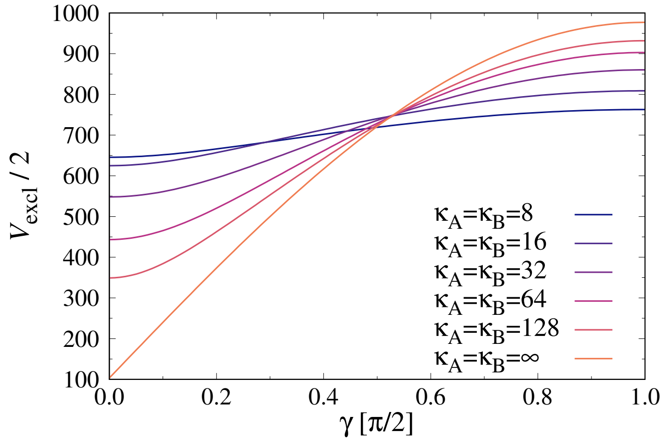


FIG. 1. Excluded volume $V_{\rm excl}$ between two (semiflxible) chains with $N = 32$ as a function of their relative orientation $\gamma$.

mers converges rather slowly to the corresponding limiting behavior of a pair of hard rods, we note from the Kratky-Porod model, that for $\ell_{\rm p} \gg L$ the average squared end-to-end distance of the semiflexible polymer is $R_{\rm e}^2 = L^2(1-3L/\ell_{\rm p})$. So we expect that for $\gamma = \pi/2$ the excluded volume of a pair of chains is reduced by an analogous factor. While for a pair of rods $\gamma = 0$ means that their orientation vectors are strictly parallel, this is not so for a pair of semiflexible polymers when we consider bond vectors. Note that the bond vectors deviate from the long axis of the polymer by an angle $\alpha \sim \sqrt{L/\ell_{\rm p}}$.[6] Figure 1 shows $V_{\rm excl}$ for a pair of semiflexible chains with $N = 32$ and various stiffnesses $\kappa_{\rm A} = \kappa_{\rm B}$, and it is interesting to see that indeed the excluded volume shows such a variation for $\gamma = \pi/2$ as well as for $\gamma = 0$. It would be desirable to use the Kratky-Porod model for an explicit calculation of the excluded volume at arbitrary angles between the chain axes, but this task is beyond the scope of the present work.

### C. Physics, limitations and mutual relation of the MD and DFT methods

MD simulations provide the exact (classical) statistical mechanics of the considered model system (defined via the chosen potentials acting on the particles), apart from statistical errors. These errors are due to the finite length of the generated trajectories, but can be reduced by more computational effort. The main limitation of the method is the finite size of the considered model system. While surface effects are eliminated by the use of periodic boundary conditions, important finite size effects could nevertheless result from interfacial excess contributions to the various densities that are recorded in cases where we study phase coexistence in the finite simulation box (see snapshots in Fig. 2 of the main manuscript). However, the analysis presented in Sec. II below provides evidence that these errors do not exceed the (small) statistical errors, and hence can be neglected. Other important finite size effects would occur in the close vicinity of the nematic-nematic critical point in the phase diagram (Fig. 2 of the main manuscript), when the correlation length of concentration fluctuations in the direction parallel to the director would become comparable to $L_z$. Although a study of such critical phenomena (possible with a subsystem finite size scaling analysis, see e.g. Ref. 7) would be interesting, we have not attempted such an analysis, since it would require significant additional computational efforts due to the slow equilibration of the system.

On the other hand, DFT does not suffer from finite size problems, but rests on three severe approximations (whose accuracy cannot be assured a priori, but only via validation by a comparison with MD a posteriori):

1. The semiflexible polymers are lumped into effective rod-like objects, with the orientations ($\omega$) of the rod as the only degrees of freedom that are kept. The effective interaction $V_{\rm excl}(\gamma)$ between two such rod-like objects is computed numerically by MC simulations (see Sec. I B above). It is only at this point that the conformational statistics of the semiflexible polymers enters the DFT calculations. These MC calculations essentially use the same model as our MD simulations, but are performed in the dilute limit and are also subject to statistical errors.

2. Since we not only wish to consider dilute solutions, but rather semidilute and concentrated solutions, the prefactor of these binary interactions between such coarse-grained semiflexible polymers is enhanced by rescaling (as explained in Ref. 6 in more detail).

3. The free energy expression for our DFT calculations (Eq. (2) in our main manuscript) is of mean field type, neglecting effects of spatial fluctuations.

For solutions containing only one type of semiflexilbe polymers, these three approximations have been shown to give reasonably accurate results for the phase transition from the isotropic to the nematic phase.[6,8] Also evidence has been presented in Ref. 6 that the slight difference between the treated models (WCA repulsion in MD, hard spheres in DFT) is not significant, as expected, since the bond lengths are almost equal ($\ell_{\rm b} = 0.97\,\sigma$ versus $\sigma$) and the bending potential is exactly the same.

For chains of different stiffness it is, however, a nontrivial question whether the small difference between the arithmetic average of two such effective potentials, $V_{\rm excl}^{\rm avg}(\gamma) = [V_{\rm excl}^{\rm AA} + V_{\rm excl}^{\rm BB}]/2$, and the actual potential, $V_{\rm excl}^{\rm AB}(\gamma)$, can be predicted with meaningful accuracy. Our results imply that *DFT can predict qualitatively correct phase diagrams*, and indeed the predicted change of topology (triple point vs. nematic-nematic critical point) does occur in our MD simulations. Thus we arrive at the important result that the DFT calculations can be

trusted also for more-component solutions of semiflexible polymers.

## II. VERIFICATION OF THERMODYNAMIC CONSISTENCY

To rule out potential finite size effects in our MD simulations originating from, e.g., the change of properties in the interfacial region and/or distortions of the nematic order by the periodic boundary conditions, we verified the thermodynamic consistency of our results using the Gibbs phase rule. When the two A-rich (A) and B-rich (B) phases coexist in our $\mathcal{N}VT$ simulations, the volume must satisfy per definition

$$V = V(\mathrm{A}) + V(\mathrm{B}). \tag{6}$$

In a two-component system, the particle numbers $\mathcal{N}_\mathrm{A}$ and $\mathcal{N}_\mathrm{B}$ then can be split into the particle numbers in the two phases

$$\mathcal{N}_\mathrm{A} = \mathcal{N}_\mathrm{A}(\mathrm{A}) + \mathcal{N}_\mathrm{A}(\mathrm{B}) \tag{7}$$
$$\mathcal{N}_\mathrm{B} = \mathcal{N}_\mathrm{B}(\mathrm{A}) + \mathcal{N}_\mathrm{B}(\mathrm{B}) \tag{8}$$

The phase diagrams (Fig. 2 in our main manuscript) are based on the four partial densities defined as $\rho_i(j) = \mathcal{N}_i(j)/V(j)$ with $i, j = \mathrm{A}, \mathrm{B}$. These four partial densities are, however, not independent from each other, but are related through the volume fraction taken by the B-rich phase $V(\mathrm{B})/V$. (Note that the volume fraction $V(\mathrm{B})/V$ is *not* the same as the mole fraction $X_\mathrm{B} = \mathcal{N}_\mathrm{B}/\mathcal{N}$.)

In terms of the partial densities of A and B in the total system, i.e. $\rho_\mathrm{A} = \mathcal{N}_\mathrm{A}/V$ and $\rho_\mathrm{B} = \mathcal{N}_\mathrm{B}/V$, the volume fraction can be cast in the following form

$$V(\mathrm{B})/V = R_1 = R_2, \tag{9}$$

with ratios $R_1$ and $R_2$ defined as

$$R_1 = [\rho_\mathrm{B} - \rho_\mathrm{B}(\mathrm{A})] \,/\, [\rho_\mathrm{B}(\mathrm{B}) - \rho_\mathrm{B}(\mathrm{A})] \tag{10}$$
$$R_2 = [\rho_\mathrm{A} - \rho_\mathrm{A}(\mathrm{A})] \,/\, [\rho_\mathrm{A}(\mathrm{B}) - \rho_\mathrm{A}(\mathrm{A})] \,. \tag{11}$$

Thus, Eq. (9) gives two independent relations for the same quantity which need to be equal if the system is in thermodynamic equilibrium. We have summarized in Table II the values of $R_1$ and $R_2$ from our MD simulations. It can be seen that the values agree with each other within the first two significant digits, hence confirming the thermodynamic consistency of our simulations.

Figure 2 shows the phase diagrams from our MD simulations in the $\rho$ *vs.* $X_\mathrm{B}$ plane. The open circles in Fig. 2 indicate the densities that we have chosen for the MD runs in the $\mathcal{N}VT$ ensemble at the chosen mole fraction $X_\mathrm{B} = 0.5$. The fact that these values lie on the corresponding tie lines connecting the coexisting phases in the $\rho$-$X_\mathrm{B}$ plane is further evidence that our results for the densities and mole fractions of these coexisting phases do not suffer from corrections due to the two interfaces between the two coexisting phases. Note that we have presented in Fig. 2 only selected two-phase equilibria, but did not attempt to locate precisely the three-phase triangle corresponding to the triple line shown in the $P - X_\mathrm{B}$ phase diagram in Fig. 2 of the main text.

| $\kappa_\mathrm{A} = 16$ | | | $\kappa_\mathrm{A} = 20$ | | |
|---|---|---|---|---|---|
| $\rho$ | $R_1$ | $R_2$ | $\rho$ | $R_1$ | $R_2$ |
| 0.250 | 0.234 | 0.236 | 0.250 | 0.289 | 0.296 |
| 0.300 | 0.403 | 0.405 | 0.275 | 0.408 | 0.414 |
| 0.350 | 0.450 | 0.454 | 0.300 | 0.485 | 0.489 |
| 0.400 | 0.484 | 0.484 | 0.325 | 0.545 | 0.548 |
| 0.425 | 0.505 | 0.504 | 0.350 | 0.614 | 0.612 |
| 0.450 | 0.559 | 0.557 | 0.600 | 0.699 | 0.700 |
| 0.475 | 0.528 | 0.529 | 0.615 | 0.520 | 0.521 |
| 0.500 | 0.504 | 0.505 | 0.630 | 0.511 | 0.516 |
| 0.550 | 0.498 | 0.495 | 0.650 | 0.506 | 0.505 |
| 0.600 | 0.483 | 0.484 | 0.670 | 0.489 | 0.491 |
| | | | 0.690 | 0.464 | 0.465 |

TABLE II. Ratios $R_1$ and $R_2$ as defined by Eqs. (10) and (11) for the MD simulations.

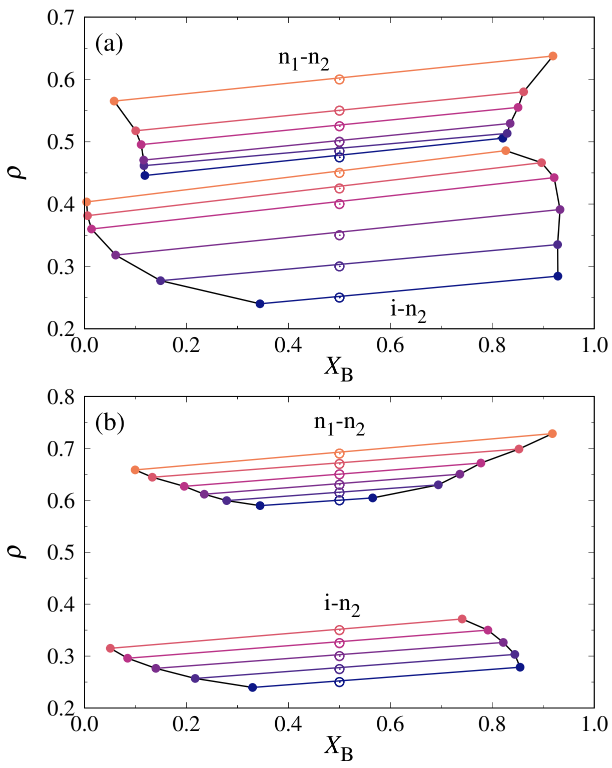


FIG. 2. Phase diagrams with tie lines in the $\rho$ *vs.* $X_\mathrm{B}$ plane for (a) $\kappa_\mathrm{A} = 16$ and (b) $\kappa_\mathrm{A} = 20$. In both panels, the left branch corresponds to $\rho_\mathrm{A} = \rho_\mathrm{A}(\mathrm{A}) + \rho_\mathrm{A}(\mathrm{B})$, while the right branch represents $\rho_\mathrm{B} = \rho_\mathrm{B}(\mathrm{B}) + \rho_\mathrm{B}(\mathrm{A})$. The open symbols indicate the point $X_\mathrm{B} = 0.5$ at the average density $\rho$ in the system.

[1] J. D. Weeks, D. Chandler, and H. C. Andersen, *Role of repulsive forces in determining the equilibrium structure of simple liquids*, J. Chem. Phys. **54**, 5237 (1971)

[2] G. S. Grest and K. Kremer, *Molecular dynamics simulation in the presence of a heat bath*, Phys. Rev. A **33**, 3628(R) (1986)

[3] A. Milchev, S. A. Egorov, K. Binder, and A. Nikoubashman, *Nematic order in solutions of semiflexible polymers: Hairpins, elastic constants, and the nematic-smectic transition*, J. Chem. Phys. **149**, 174909 (2018)

[4] H. Fynewever and A. Yethiraj, *Phase behaviour of semiflexible tangent hard sphere chains*, J. Chem. Phys. **108**, 1636-1644 (1998)

[5] J. J. de Pablo, M. Laso, and U. W. Suter, *Simulation of polyethylene above and below the melting point*, J. Chem. Phys. **96**, 2395 (1991)

[6] S. A. Egorov, A. Milchev, P. Virnau and K. Binder, *A new insight into the isotropic-nematic phase transition in lyotropic solutions of semiflexible polymers: Density-functional theory tested by molecular dynamics*, Soft Matter **12**, 4944-4959 (2016)

[7] J. Midya, S. A. Egorov, K. Binder and A. Nikoubashman, *Phase behavior of flexible and semiflexible polymers in solvents of varying quality*, J. Chem. Phys. **151**, 034902 (2019)

[8] S. A. Egorov, A. Milchev and K. Binder, *Anomalous fluctuations of nematic order in solutions of semiflexible polymers*, Phys. Rev. Lett. **116**, 187801 (2016)
